# Supplementary material for: Linking Representations with Multimodal Contrastive Learning
Source: arXiv:2304.03464 source file (2024-06-21)
Supplement: Supplementary file 1 [file additional_newspaper_results.tex]

\begin{table}[ht]
    \centering
    %\resizebox{\linewidth}{!}{
    \begin{threeparttable}
       \begin{tabular}{lc}
      \toprule
       & ARI \\
\cmidrule{1-2}

\multicolumn{2}{l}
{\textbf{\textit{Panel A: Zero-shot CLIP}}} \\
Visual Linking & 	
0.182 \\
Language Linking   & 0.291 \\
Multimodal Linking  & 0.314 \\

\multicolumn{2}{l}
{\textbf{\textit{Panel B: Only Supervised Training}}} \\
Visual Linking & 	
 0.200 \\
Language Linking   & 0.303 \\
Multimodal Linking  & 	
0.559 \\     \bottomrule 
    \end{tabular}
    \end{threeparttable}
 %}
    \caption{Noisy Duplicate Ablations: This table reports the adjusted rand index for detecting noisy duplicated image-caption pairs in a historical newspaper corpus, using CLIP off-the-shelf (Panel A) and using only supervised training, with no language-image pre-training (Panel B).}
      \label{add_news_matching_results}
\end{table}
